# Supplementary material for: Birds have four legs?! NumerSense: Probing Numerical Commonsense Knowledge of Pre-trained Language Models
Source: arXiv:2005.00683 source file (2020-09-18)
Supplement: Supplementary file 1 [file appendix.tex]

\appendix

\section{Experimental details}
Our framework is based on HuggingFace transformers\footnote{\url{https://github.com/huggingface/transformers}} and its extension HappyTransformer\footnote{\url{https://pypi.org/project/happytransformer/}}.
All the tested models are directly downloaded from huggingface port and the size of the model parameters are as follows:
\begin{itemize}
    \item GPT-2: 345M
    \item BERT-base and RoBERTa-base: 110M
    \item BERT-large and RoBERTa-large: 340M
\end{itemize}
Note that we used uncased versions for BERT.

We fine-tune BERT and RoBERTa large by modifying the official fine-tuning scripts and change the masking strategy to only mask number words in the sentences at all the time.
The training time of both models are less than 5 hours on a single Titan 1080 Ti GPU (with --fp16 optimization). 
The manually tuned hyper-parameters are as follows:
\begin{itemize}
    \item per\_gpu\_batch\_size = \{16, 32, \textbf{64}, 128\}
    \item learning\_rate = \{8e-5, \textbf{5e-5}, 3e-5, 1e-5\}
    \item weight\_decay = \{\textbf{0.0}, 0.1, 0.2\}
    \item adam\_epsilon = \textbf{1e-8}
    \item max\_grad\_norm = \textbf{1}
    \item num\_train\_epochs 20 
\end{itemize}

We highlight the bound of the manual hyper-parameter tuning, and we also do early stop by evaluating the models on a set of number-contained Wikipedia sentences, which are collected in the same way of Section~\ref{ssec:ds} with lower quality.
We found that the models usually converge after epoch 5, and this also holds for evaluation on test set.
